# Supplementary material for: Race for Quantum Advantage using Random Circuit Sampling
Source: arXiv:2211.13267 source file (2022-11-23)
Supplement: Supplementary file 1 [file SM5_RandomTest_Kalachev_Pan.pdf]

Test Data File:/home/soh/Desktop/Q_Advantage/Kalachev/Kalachev_samples_m12_f0_02.txt

| Type of Test | | | P-Value | Conclusion |
|---|---|---|---|---|
| 01. Frequency Test (Monobit) | | | 0.4764647760211399 | Random |
| 02. Frequency Test within a Block | | | 0.21344408868047735 | Random |
| 03. Run Test | | | 0.6308667935708817 | Random |
| 04. Longest Run of Ones in a Block | | | 0.3236366520845152 | Random |
| 05. Binary Matrix Rank Test | | | 0.521670870053001 | Random |
| 06. Discrete Fourier Transform (Spectral) Test | | | 0.9341778199756322 | Random |
| 07. Non-Overlapping Template Matching Test | | | 0.7037740823650909 | Random |
| 08. Overlapping Template Matching Test | | | 0.36843103345819184 | Random |
| 09. Maurer's Universal Statistical test | | | 0.8128577030067433 | Random |
| 10. Linear Complexity Test | | | 0.9137783567700142 | Random |
| 11. Serial test: | | | | |
| | | | 0.061149134291070724 | Random |
| | | | 0.12284412750640619 | Random |
| 12. Approximate Entropy Test | | | 0.3468070684337232 | Random |
| 13. Cummulative Sums (Forward) Test | | | 0.8694388017798453 | Random |
| 14. Cummulative Sums (Reverse) Test | | | 0.512251231818323 | Random |
| 15. Random Excursions Test: | | | | |
| | State | Chi Squared | P-Value | Conclusion |
| | -4 | 3.968657150936274 | 0.5539373482919261 | Random |
| | -3 | 3.9099879598662186 | 0.5624470250933297 | Random |
| | -2 | 2.6697634088938433 | 0.7507389625417105 | Random |
| | -1 | 4.959866220735786 | 0.4207978049618142 | Random |
| | +1 | 1.5418060200668897 | 0.9081955736195303 | Random |
| | +2 | 3.384739254304472 | 0.6408952021373548 | Random |
| | +3 | 3.9997913043478275 | 0.5494459988912636 | Random |
| | +4 | 3.483809003773511 | 0.625838936024486 | Random |
| 16. Random Excursions Variant Test: | | | | |
| | State | COUNTS | P-Value | Conclusion |
| | -9.0 | 338 | 0.6989022403517948 | Random |
| | -8.0 | 314 | 0.8741588958050495 | Random |
| | -7.0 | 284 | 0.8649115702567244 | Random |
| | -6.0 | 259 | 0.6218793101786622 | Random |
| | -5.0 | 289 | 0.891576110765103 | Random |
| | -4.0 | 323 | 0.7106771560813343 | Random |
| | -3.0 | 306 | 0.8981367326247249 | Random |
| | -2.0 | 286 | 0.7589005304123926 | Random |
| | -1.0 | 294 | 0.8379899799745315 | Random |
| | +1.0 | 276 | 0.34694067113894966 | Random |
| | +2.0 | 237 | 0.1432497748490905 | Random |
| | +3.0 | 217 | 0.13371551809318777 | Random |
| | +4.0 | 220 | 0.22207344262264084 | Random |
| | +5.0 | 218 | 0.26954450996408963 | Random |
| | +6.0 | 242 | 0.4821842620195139 | Random |
| | +7.0 | 241 | 0.5106551134617632 | Random |
| | +8.0 | 202 | 0.3057511299615784 | Random |
| | +9.0 | 221 | 0.4391641172706955 | Random |

Test Data File:/home/soh/Desktop/Q_Advantage/Kalachev/Kalachev_samples_m14_f0_02.txt

| Type of Test | | | P-Value | Conclusion |
|---|---|---|---|---|
| 01. Frequency Test (Monobit) | | | 0.36812025069351906 | Random |
| 02. Frequency Test within a Block | | | 0.5990050126598513 | Random |
| 03. Run Test | | | 0.27872370809503944 | Random |
| 04. Longest Run of Ones in a Block | | | 0.9734077333463553 | Random |
| 05. Binary Matrix Rank Test | | | 0.675959832222133 | Random |
| 06. Discrete Fourier Transform (Spectral) Test | | | 0.6463551955394902 | Random |
| 07. Non-Overlapping Template Matching Test | | | 0.046523744516345174 | Random |
| 08. Overlapping Template Matching Test | | | 0.7945618963945935 | Random |
| 09. Maurer's Universal Statistical test | | | 0.6919599594792027 | Random |
| 10. Linear Complexity Test | | | 0.46060787586617724 | Random |
| 11. Serial test: | | | | |
| | | | 0.6140804852141764 | Random |
| | | | 0.4437895055934931 | Random |
| 12. Approximate Entropy Test | | | 0.6378590153718529 | Random |
| 13. Cummulative Sums (Forward) Test | | | 0.32597464591167397 | Random |
| 14. Cummulative Sums (Reverse) Test | | | 0.239885966313531 | Random |
| 15. Random Excursions Test: | | | | |
| | State | Chi Squared | P-Value | Conclusion |
| | -4 | 4.7191886934958465 | 0.45110246764886486 | Random |
| | -3 | 4.647168149882899 | 0.4604374521359824 | Random |
| | -2 | 4.3909657771224255 | 0.49460300631740384 | Random |
| | -1 | 2.9797033567525366 | 0.7031151430976014 | Random |
| | +1 | 11.587041373926619 | 0.04090600744668136 | Random |
| | +2 | 2.2758358149979276 | 0.8098093203523501 | Random |
| | +3 | 1.5749882903981258 | 0.9042573312321506 | Random |
| | +4 | 1.2239367476666143 | 0.9425604486819531 | Random |
| 16. Random Excursions Variant Test: | | | | |
| | State | COUNTS | P-Value | Conclusion |
| | -9.0 | 1468 | 0.3702311954986752 | Random |
| | -8.0 | 1430 | 0.44721537479102025 | Random |
| | -7.0 | 1422 | 0.4397558060002761 | Random |
| | -6.0 | 1426 | 0.38773175694720885 | Random |
| | -5.0 | 1449 | 0.26856852855316427 | Random |
| | -4.0 | 1446 | 0.2179123630378087 | Random |
| | -3.0 | 1407 | 0.2655974678979497 | Random |
| | -2.0 | 1352 | 0.41802256278126726 | Random |
| | -1.0 | 1333 | 0.30426085776276945 | Random |
| | +1.0 | 1256 | 0.6213676320840416 | Random |
| | +2.0 | 1265 | 0.8551880712099779 | Random |
| | +3.0 | 1280 | 0.9929504751436469 | Random |
| | +4.0 | 1301 | 0.8812812116146737 | Random |
| | +5.0 | 1267 | 0.9265414492766206 | Random |
| | +6.0 | 1225 | 0.7386952848776749 | Random |
| | +7.0 | 1159 | 0.5038172515892158 | Random |
| | +8.0 | 1067 | 0.2749923173193948 | Random |
| | +9.0 | 1026 | 0.22175556272566965 | Random |

Test Data File:/home/soh/Desktop/Q_Advantage/Kalachev/Kalachev_samples_m16_f0_02.txt

| Type of Test | | | P-Value | Conclusion |
|---|---|---|---|---|
| 01. Frequency Test (Monobit) | | | 0.8446101659967438 | Random |
| 02. Frequency Test within a Block | | | 0.1313095540114925 | Random |
| 03. Run Test | | | 0.6114263887514859 | Random |
| 04. Longest Run of Ones in a Block | | | 0.1931679889686314 | Random |
| 05. Binary Matrix Rank Test | | | 0.022916094922390124 | Random |
| 06. Discrete Fourier Transform (Spectral) Test | | | 0.6931417581917918 | Random |
| 07. Non-Overlapping Template Matching Test | | | 0.2593392856825376 | Random |
| 08. Overlapping Template Matching Test | | | 0.9976883347701309 | Random |
| 09. Maurer's Universal Statistical test | | | 0.5688525819051272 | Random |
| 10. Linear Complexity Test | | | 0.898864436013856 | Random |
| 11. Serial test: | | | | |
| | | | 0.17833073938631794 | Random |
| | | | 0.5997502310028316 | Random |
| 12. Approximate Entropy Test | | | 0.7560149294104068 | Random |
| 13. Cummulative Sums (Forward) Test | | | 0.20874940761590788 | Random |
| 14. Cummulative Sums (Reverse) Test | | | 0.1375179145566432 | Random |
| 15. Random Excursions Test: | | | | |
| | State | Chi Squared | P-Value | Conclusion |
| | -4 | 0.851260387536939 | 0.9736492409420993 | Random |
| | -3 | 1.4033714285714292 | 0.9239441197448341 | Random |
| | -2 | 2.0121693121693123 | 0.8474586300616996 | Random |
| | -1 | 6.745238095238095 | 0.2402871316448323 | Random |
| | +1 | 9.983333333333334 | 0.07570886846223805 | Random |
| | +2 | 6.676954732510288 | 0.24579522761536815 | Random |
| | +3 | 6.718445714285711 | 0.24243595469941376 | Random |
| | +4 | 3.749247337418933 | 0.5860525864188788 | Random |
| 16. Random Excursions Variant Test: | | | | |
| | State | COUNTS | P-Value | Conclusion |
| | -9.0 | 699 | 0.40409272267395846 | Random |
| | -8.0 | 672 | 0.28991845394257 | Random |
| | -7.0 | 705 | 0.36098085015452963 | Random |
| | -6.0 | 773 | 0.6221113145306909 | Random |
| | -5.0 | 788 | 0.6723754961004647 | Random |
| | -4.0 | 768 | 0.5067287122720537 | Random |
| | -3.0 | 814 | 0.7766531265771661 | Random |
| | -2.0 | 794 | 0.5170162581476525 | Random |
| | -1.0 | 769 | 0.08323393139707815 | Random |
| | +1.0 | 848 | 0.8452520242196513 | Random |
| | +2.0 | 790 | 0.48124894729058065 | Random |
| | +3.0 | 740 | 0.27523352407483437 | Random |
| | +4.0 | 720 | 0.2684813240895787 | Random |
| | +5.0 | 710 | 0.2904088766853078 | Random |
| | +6.0 | 708 | 0.33154413922629256 | Random |
| | +7.0 | 686 | 0.297381995349405 | Random |
| | +8.0 | 623 | 0.1716342354674001 | Random |
| | +9.0 | 559 | 0.09636228826002577 | Random |

Test Data File:/home/soh/Desktop/Q_Advantage/Kalachev/Kalachev_samples_m18_f0_02.txt

| Type of Test | | | P-Value | Conclusion |
|---|---|---|---|---|
| 01. Frequency Test (Monobit) | | | 0.5326275850684048 | Random |
| 02. Frequency Test within a Block | | | 0.1610434905416323 | Random |
| 03. Run Test | | | 0.41357937736213857 | Random |
| 04. Longest Run of Ones in a Block | | | 0.5860464260985603 | Random |
| 05. Binary Matrix Rank Test | | | 0.7506657464669498 | Random |
| 06. Discrete Fourier Transform (Spectral) Test | | | 0.8185458083820434 | Random |
| 07. Non-Overlapping Template Matching Test | | | 0.7229265843266949 | Random |
| 08. Overlapping Template Matching Test | | | 0.8075937247214546 | Random |
| 09. Maurer's Universal Statistical test | | | 0.2061918781765083 | Random |
| 10. Linear Complexity Test | | | 0.09263452893275469 | Random |
| 11. Serial test: | | | | |
| | | | 0.9948613514719569 | Random |
| | | | 0.983110914316642 | Random |
| 12. Approximate Entropy Test | | | 0.9041319130893657 | Random |
| 13. Cummulative Sums (Forward) Test | | | 0.8995316019481437 | Random |
| 14. Cummulative Sums (Reverse) Test | | | 0.372854700954095 | Random |
| 15. Random Excursions Test: | | | | |
| | State | Chi Squared | P-Value | Conclusion |
| | -4 | 2.9091220607858497 | 0.713994163200854 | Random |
| | -3 | 1.7901353028064975 | 0.8773542766236688 | Random |
| | -2 | 2.4326458413115235 | 0.7866028011747018 | Random |
| | -1 | 3.0945347119645494 | 0.6854140043414926 | Random |
| | +1 | 5.738552437223043 | 0.33249575659109676 | Random |
| | +2 | 1.5406933274978574 | 0.9083265808820561 | Random |
| | +3 | 3.371568685376662 | 0.6429036256167626 | Random |
| | +4 | 2.7447346225138833 | 0.7392684325323876 | Random |
| 16. Random Excursions Variant Test: | | | | |
| | State | COUNTS | P-Value | Conclusion |
| | -9.0 | 895 | 0.1507500243065136 | Random |
| | -8.0 | 941 | 0.06395971917401909 | Random |
| | -7.0 | 934 | 0.05273308036219564 | Random |
| | -6.0 | 896 | 0.07273670815467283 | Random |
| | -5.0 | 798 | 0.2730299282585611 | Random |
| | -4.0 | 714 | 0.7039065884595109 | Random |
| | -3.0 | 684 | 0.9322014931354055 | Random |
| | -2.0 | 667 | 0.8753216391487707 | Random |
| | -1.0 | 675 | 0.9566542088377044 | Random |
| | +1.0 | 654 | 0.5319347057250245 | Random |
| | +2.0 | 678 | 0.987481500312186 | Random |
| | +3.0 | 750 | 0.37496354295666523 | Random |
| | +4.0 | 741 | 0.5109316119122291 | Random |
| | +5.0 | 693 | 0.884757944370298 | Random |
| | +6.0 | 709 | 0.7931618467230598 | Random |
| | +7.0 | 705 | 0.8328514156163357 | Random |
| | +8.0 | 682 | 0.9720123770523453 | Random |
| | +9.0 | 703 | 0.8639313660429062 | Random |

Test Data File:/home/soh/Desktop/Q_Advantage/Kalachev/Kalachev_samples_m20_f0_002.txt

| Type of Test | | | P-Value | Conclusion |
|---|---|---|---|---|
| 01. Frequency Test (Monobit) | | | 0.8103302566044084 | Random |
| 02. Frequency Test within a Block | | | 0.6451226658545621 | Random |
| 03. Run Test | | | 0.013814242475825765 | Random |
| 04. Longest Run of Ones in a Block | | | 0.6247694555788041 | Random |
| 05. Binary Matrix Rank Test | | | 0.46079850859791666 | Random |
| 06. Discrete Fourier Transform (Spectral) Test | | | 0.2912824828600983 | Random |
| 07. Non-Overlapping Template Matching Test | | | 0.7388810101607451 | Random |
| 08. Overlapping Template Matching Test | | | 0.4811398314086006 | Random |
| 09. Maurer's Universal Statistical test | | | 0.38185010101348194 | Random |
| 10. Linear Complexity Test | | | 0.02706655069192337 | Random |
| 11. Serial test: | | | | |
| | | | 0.9922192227949157 | Random |
| | | | 0.9968791142357275 | Random |
| 12. Approximate Entropy Test | | | 0.8692002925458828 | Random |
| 13. Cummulative Sums (Forward) Test | | | 0.6754847276886258 | Random |
| 14. Cummulative Sums (Reverse) Test | | | 0.5930631791010212 | Random |
| 15. Random Excursions Test: | | | | |
| | State | Chi Squared | P-Value | Conclusion |
| | -4 | 3.7030998988516686 | 0.5929027181539119 | Random |
| | -3 | 4.6970857142857145 | 0.4539544969357938 | Random |
| | -2 | 3.757936507936508 | 0.5847662473700188 | Random |
| | -1 | 2.160714285714286 | 0.826489874866238 | Random |
| | +1 | 5.446428571428571 | 0.3638559475997174 | Random |
| | +2 | 5.193562610229276 | 0.3927173469584401 | Random |
| | +3 | 1.490428571428571 | 0.9141717048981742 | Random |
| | +4 | 2.0493841851609447 | 0.8422704699599011 | Random |
| 16. Random Excursions Variant Test: | | | | |
| | State | COUNTS | P-Value | Conclusion |
| | -9.0 | 167 | 0.37277891115288564 | Random |
| | -8.0 | 189 | 0.18405385732510526 | Random |
| | -7.0 | 186 | 0.1702779546098222 | Random |
| | -6.0 | 182 | 0.15848353257474201 | Random |
| | -5.0 | 185 | 0.10398386228758541 | Random |
| | -4.0 | 182 | 0.07709987174354177 | Random |
| | -3.0 | 169 | 0.0885305029552949 | Random |
| | -2.0 | 143 | 0.23175472441333744 | Random |
| | -1.0 | 126 | 0.3495748061232983 | Random |
| | +1.0 | 112 | 1.0 | Random |
| | +2.0 | 123 | 0.6713220917153243 | Random |
| | +3.0 | 113 | 0.9761621859960805 | Random |
| | +4.0 | 81 | 0.4337045002397064 | Random |
| | +5.0 | 74 | 0.39737020128916656 | Random |
| | +6.0 | 67 | 0.36464437123377547 | Random |
| | +7.0 | 38 | 0.1702779546098222 | Random |
| | +8.0 | 34 | 0.17842256834886872 | Random |
| | +9.0 | 42 | 0.2566450312893328 | Random |

```
Test Data File:/home/soh/Desktop/Q_Advantage/Kalachev/Kalachev_spoofing_m20_tmp.txt


Type of Test                                        P-Value                 Conclusion
01. Frequency Test (Monobit)                        0.0                     Non-Random
02. Frequency Test within a Block                   0.0                     Non-Random
03. Run Test                                        0.0                     Non-Random
04. Longest Run of Ones in a Block                  4.4003844943604805e-220 Non-Random
05. Binary Matrix Rank Test                         0.2527770448278441      Random
06. Discrete Fourier Transform (Spectral) Test      0.0                     Non-Random
07. Non-Overlapping Template Matching Test          0.0                     Non-Random
08. Overlapping Template Matching Test              0.0                     Non-Random
09. Maurer's Universal Statistical test             0.0                     Non-Random
10. Linear Complexity Test                          0.9244890828213794      Random
11. Serial test:
                                                    0.0                     Non-Random
                                                    0.0                     Non-Random
12. Approximate Entropy Test                        0.0                     Non-Random
13. Cummulative Sums (Forward) Test                 0.0                     Non-Random
14. Cummulative Sums (Reverse) Test                 0.0                     Non-Random
15. Random Excursions Test:
                State       Chi Squared             P-Value                 Conclusion
                -4          63.0                    2.9111549198896303e-12  Non-Random
                -3          35.0                    1.5046506621757205e-06  Non-Random
                -2          15.0                    0.010362337915786429    Random
                -1          3.0                     0.6999858358786276      Random
                +1          1.0                     0.9625657732472964      Random
                +2          0.3333333333333333      0.9969687632568645      Random
                +3          0.2                     0.9991138612111875      Random
                +4          0.14285714285714285     0.9996100613790039      Random
16. Random Excursions Variant Test:
                State       COUNTS                  P-Value                 Conclusion
                -9.0        1                       1.0                     Random
                -8.0        1                       1.0                     Random
                -7.0        1                       1.0                     Random
                -6.0        1                       1.0                     Random
                -5.0        1                       1.0                     Random
                -4.0        1                       1.0                     Random
                -3.0        1                       1.0                     Random
                -2.0        1                       1.0                     Random
                -1.0        1                       1.0                     Random
```

Test Data File:/home/soh/Desktop/Manuscripts/Paper1_RCS/Data/Kalachev/Pan.samples_metropolis.txt

| Type of Test | P-Value | Conclusion |
|---|---|---|
| 01. Frequency Test (Monobit) | 2.0585601824114782e-169 | Non-Random |
| 02. Frequency Test within a Block | 9.00880750481587e-70 | Non-Random |
| 03. Run Test | 0.0 | Non-Random |
| 04. Longest Run of Ones in a Block | 2.3304231212946727e-06 | Non-Random |
| 05. Binary Matrix Rank Test | 0.07752966451590863 | Random |
| 06. Discrete Fourier Transform (Spectral) Test | 0.0 | Non-Random |
| 07. Non-Overlapping Template Matching Test | 0.0 | Non-Random |
| 08. Overlapping Template Matching Test | 8.621989047751373e-17 | Non-Random |
| 09. Maurer's Universal Statistical test | 0.0 | Non-Random |
| 10. Linear Complexity Test | 0.44581754606703217 | Random |
| 11. Serial test: | | |
| | 0.0 | Non-Random |
| | 6.923147645901766e-08 | Non-Random |
| 12. Approximate Entropy Test | 0.0 | Non-Random |
| 13. Cummulative Sums (Forward) Test | 6.2416452221212e-170 | Non-Random |
| 14. Cummulative Sums (Reverse) Test | 1.0292800912056217e-169 | Non-Random |

15. Random Excursions Test:

| State | Chi Squared | P-Value | Conclusion |
|---|---|---|---|
| -4 | 63.0 | 2.9111549198896303e-12 | Non-Random |
| -3 | 35.0 | 1.5046506621757205e-06 | Non-Random |
| -2 | 15.0 | 0.010362337915786429 | Random |
| -1 | 3.0 | 0.6999858358786276 | Random |
| +1 | 1.0 | 0.9625657732472964 | Random |
| +2 | 0.3333333333333333 | 0.9969687632568645 | Random |
| +3 | 0.2 | 0.9991138612111875 | Random |
| +4 | 0.14285714285714285 | 0.9996100613790039 | Random |

16. Random Excursions Variant Test:

| State | COUNTS | P-Value | Conclusion |
|---|---|---|---|
| -9.0 | 1 | 1.0 | Random |
| -8.0 | 1 | 1.0 | Random |
| -7.0 | 1 | 1.0 | Random |
| -6.0 | 1 | 1.0 | Random |
| -5.0 | 1 | 1.0 | Random |
| -4.0 | 1 | 1.0 | Random |
| -3.0 | 1 | 1.0 | Random |
| -2.0 | 1 | 1.0 | Random |
| -1.0 | 1 | 1.0 | Random |
